# Supplementary material for: Adaptive Prompting: Ad-hoc Prompt Composition for Social Bias Detection
Source: arXiv:2502.06487 source file (2025-02-10)
Supplement: Supplementary file 1 [file figure-network-plots-appendix.tex]

\begin{figure*}
    \centering
    \begin{minipage}[c]{0.14\linewidth}
    \phantom{a}
    \end{minipage}
    \hfill
    \begin{minipage}[c]{0.40\linewidth}
       \centering\textbf{Stereoset}
    \end{minipage}
    \hfill
    \begin{minipage}[c]{0.40\linewidth}
        \centering\textbf{SBIC}
    \end{minipage}
    \\[1em]
    \begin{minipage}[c]{0.14\linewidth}
    \textbf{Mistral}
    \end{minipage}
    \hfill
    \begin{minipage}[c]{0.40\linewidth}       \centering\includegraphics[width=\linewidth]{network_stereoset_mistral.pdf}
    \end{minipage}
    \hfill
    \begin{minipage}[c]{0.40\linewidth}
        \centering\includegraphics[width=\linewidth]{network_sbic_mistral.pdf}
    \end{minipage}
    \\[1em]
    \begin{minipage}[c]{0.14\linewidth}
    \textbf{Llama~3}
    \end{minipage}
    \hfill
    \begin{minipage}[c]{0.40\linewidth}
       \centering\includegraphics[width=\linewidth]{network_stereoset_llama3.pdf}
    \end{minipage}
    \hfill
    \begin{minipage}[c]{0.40\linewidth}
        \centering\includegraphics[width=\linewidth]{network_sbic_llama3.pdf}
    \end{minipage}
    \\[1em]
    \begin{minipage}[c]{0.14\linewidth}
    \textbf{Command-R}
    \end{minipage}
    \hfill
    \begin{minipage}[c]{0.40\linewidth}
       \centering\includegraphics[width=\linewidth]{network_stereoset_command-r.pdf}
    \end{minipage}
    \hfill
    \begin{minipage}[c]{0.40\linewidth}
        \centering\includegraphics[width=\linewidth]{network_sbic_command-r.pdf}
    \end{minipage}

    \caption{Network plots of the SIs for different variants of the prompt composition game revealing \textbf{unique interaction structures} among the models and datasets. The size of the nodes represents the strengths of first-order interactions and the width and transparency of the lines denotes the strengths of second-order interactions. Red color denotes positive interaction (increasing the performance), and blue color denotes negative interaction (decreasing the performance).}
    \label{fig_network_plots_appendix}
\end{figure*}
